# Supplementary material for: A search for signatures of Europa's atmosphere and plumes in Galileo charged particle data
Source: arXiv:1812.11215 source file (2018-12-28)
Supplement: Supplementary file 1 [file data_overview.tex]

%\section{Overview of the data}
%\label{app_overview}
%
%In this Appendix an overview of the EPD, PLS and MAG data collected during the Europa flybys of Galileo is provided. Data products that are presented are the count rates in the EPD E, A, TP, TO and TS channels. For PLS both the differential flux, the count rate, the plasma density and magnitude of the velocity are presented. For MAG the magnitude of the mangetic field is shown. The flybys data are shown in sequential order in Figures \ref{img_E4_all} to \ref{img_E26_all}. In every figure the solid vertical line indicates the time of the closest approach.
%
%\begin{figure}[h]
%  \centering
%  %\includegraphics[width=1.0\textwidth]{data_multi_instrument/ql_19961219_062059.pdf}
%  \includegraphics[width=1.0\textwidth]{data_multi_instrument/E4.pdf}
%  \caption{E4 flyby data, dashed vertical lines indicate the geometrical wake. The dotted lines indicate the region in which \cite{Paterson1999} reports deflection of the corotational plasma based on PLS data.}
%  \label{img_E4_all}
%\end{figure}
%
%\begin{figure}[h]
%  \centering
%  %\includegraphics[width=1.0\textwidth]{data_multi_instrument/ql_19970220_163459.pdf}
%    \includegraphics[width=1.0\textwidth]{data_multi_instrument/E6.pdf}
%  \caption{E6 flyby data. The dotted lines indicate the region in which \cite{Paterson1999} reports deflection of the corotational plasma based on PLS data.}
%  \label{img_E6_all}
%\end{figure}
%
%\begin{figure}[h]
%  \centering
%  %\includegraphics[width=1.0\textwidth]{data_multi_instrument/ql_19971106_200459.pdf}
%  \includegraphics[width=1.0\textwidth]{data_multi_instrument/E11.pdf}
%  \caption{E11 flyby data, dashed vertical lines indicate the geometrical wake.}
%  \label{img_E11_all}
%\end{figure}
%
%\begin{figure}[h]
%  \centering
%  %\includegraphics[width=1.0\textwidth]{data_multi_instrument/ql_19971216_114000.pdf}
%  \includegraphics[width=1.0\textwidth]{data_multi_instrument/E12.pdf}
%  \caption{E12 flyby data. The dotted lines indicate the region during which the direction of the corotational plasma changes according to our analysis of the PLS data, see Chapter \ref{ch_comparison}. \cite{Jia2018} reports a change in magnetic field direction between the first dotted line and the closet approach (solid line), possibly related to a plume.}
%  \label{img_E12_all}
%\end{figure}
%
%\begin{figure}[h]
%  \centering
%  %\includegraphics[width=1.0\textwidth]{data_multi_instrument/ql_19980329_130000.pdf}
%  \includegraphics[width=1.0\textwidth]{data_multi_instrument/E14.pdf}
%  \caption{E14 flyby data}
%  \label{img_E14_all}
%\end{figure}
%
%\begin{figure}[h]
%  \centering
%  %\includegraphics[width=1.0\textwidth]{data_multi_instrument/ql_19980531_203959.pdf}
%   \includegraphics[width=1.0\textwidth]{data_multi_instrument/E15.pdf}
%  \caption{E15 flyby data, dashed vertical lines indicate the geometrical wake.}
%  \label{img_E15_all}
%\end{figure}
%
%\begin{figure}[h]
%  \centering
%  %\includegraphics[width=1.0\textwidth]{data_multi_instrument/ql_19990201_014500.pdf}
%  \includegraphics[width=1.0\textwidth]{data_multi_instrument/E19.pdf}   \caption{E19 flyby data}
%  \label{img_E19_all}
%\end{figure}
%
%\begin{figure}[h]
%  \centering
%  %\includegraphics[width=1.0\textwidth]{data_multi_instrument/ql_20000103_172000.pdf}
%  \includegraphics[width=1.0\textwidth]{data_multi_instrument/E26.pdf}
%  \caption{E26 flyby data}
%  \label{img_E26_all}
%\end{figure}
%
%
%%\subsection{Upstream-downstream wake flybys}
%%
%%This section describes the flybys that passed from upstream to downstream, through the wake of Europa. These flybys are E4 (Figure \ref{img_E4_all}), E11 (Figure \ref{img_E11_all}) and E15 (Figure \ref{img_E15_all}).
%%
%%\subsection{Upstream-downstream non-wake flybys}
%%This section describes the flybys that passed from upstream to downstream, but not through the wake of Europa. These flybys are E6 (Figure \ref{img_E6_all}), E12 (Figure \ref{img_E12_all}), E14 (Figure \ref{img_E14_all}) and E19 (Figure \ref{img_E19_all}).
%%
%%\subsection{Upstream flybys - E26}
%%In this Section the E26 flyby data is shown, this flyby passed fully upstream of Europa (Figure \ref{img_E26_all}).
%
%
